# Supplementary material for: Ultra-Bright Electron Bunch Injection in a Plasma Wakefield Driven by a Superluminal Flying Focus Electron Beam
Source: arXiv:2108.00030 ancillary file (2022-04-24)
Supplement: Supplementary file 1 [file supplemental_material.pdf]

# Supplemental Material for “Ultra-bright Electron Bunch Injection in a Plasma Wakefield Driven by a Superluminal Flying Focus Electron Beam”

## VELOCITY OF THE FLYING FOCUS

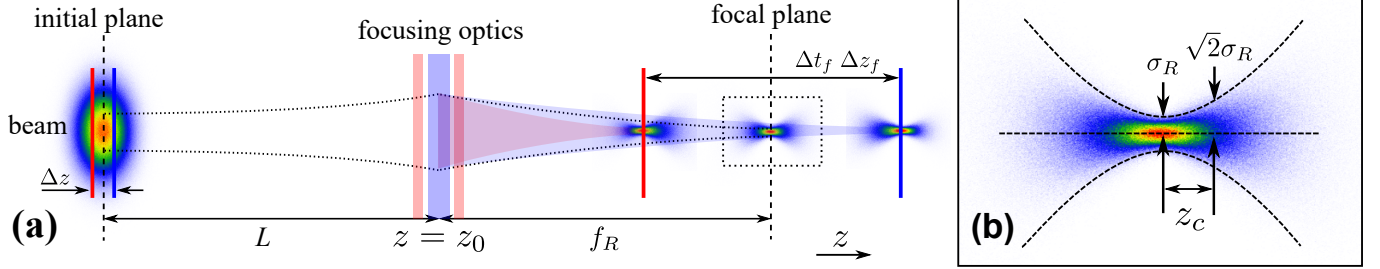

FIG. 1. (a) Schematic of focusing a negative-chirped beam. (b) Typical density distribution of an FF beam at the focal plane (zoom-in plot of the region in the dashed-line box). A linear energy chirp was used to generate this plot.

The velocity of the beam peak density (flying focus, FF) can be derived by examining two slices within the beam located at  $z$  and  $z + \Delta z$  before traveling through the focusing lens as denoted by the red and blue solid lines in Fig. 1(a). From the red to the blue slice, we assume the Lorentz factor, momentum and velocity increase from  $(\gamma, p, \beta)$  to  $(\gamma + \Delta\gamma, p + \Delta p, \beta + \Delta\beta)$  due to the energy chirp. The focal lengths of the two slices are  $f$  and  $f(1 + \Delta p/p)$  respectively since the focal length is proportional to beam momentum. The spacing between the focal planes of the two slices is therefore,

$$\Delta z_f = f \left( 1 + \frac{\Delta p}{p} \right) - f = f \frac{\Delta p}{p} \quad (1)$$

and the time difference to reach the focal planes is given by

$$c\Delta t_f = \frac{f(1 + \Delta p/p) - \Delta z + L}{\beta + \Delta\beta} - \frac{f + L}{\beta} = \frac{1}{\beta(\beta + \Delta\beta)} \left( f\beta \frac{\Delta p}{p} - f\Delta\beta - L\Delta\beta - \beta\Delta z \right), \quad (2)$$

where the particle velocity  $\beta$  is approximately equal to the longitudinal velocity  $\beta_z$  since the transverse velocity  $\beta_\perp$  is negligibly small. Thus, we have  $\beta^2 = 1 - 1/\gamma^2$  and  $\Delta\beta = \Delta\gamma/(\beta\gamma^3) = \Delta p/\gamma^3$  and the velocity of the flying focus can be written as

$$\beta_f = \frac{\Delta z_f}{c\Delta t_f} = \frac{f\beta \frac{\Delta p}{p} (\beta + \Delta\beta)}{f\beta \frac{\Delta p}{p} - f\Delta\beta - L\Delta\beta - \beta\Delta z} \quad (3)$$

$$\stackrel{\Delta z \rightarrow 0}{=} \frac{\beta}{1 - \frac{p}{f} \left( \frac{dp}{dz} \right)^{-1} - \left( 1 + \frac{L}{f} \right) \frac{1}{\gamma^2}}$$

Note that  $p/f = p_R/f_R$  where the subscript “R” denotes the reference particle, and  $dp/dz = -dp/d\xi$  for a given time. Therefore, Eq. (3) can be rewritten as

$$\beta_f = \frac{\beta}{1 + \frac{p_R}{f_R} \left( \frac{dp}{d\xi} \right)^{-1} - \left( 1 + \frac{L}{f} \right) \frac{1}{\gamma^2}} \simeq 1 - \frac{p_R}{f_R} \left( \frac{dp}{d\xi} \right)^{-1} + \frac{1}{2\gamma^2} \left[ 1 + \frac{2L}{f} - \left( 3 + \frac{4L}{f} \right) \frac{p_R}{f_R} \left( \frac{dp}{d\xi} \right)^{-1} \right] + O(\gamma^{-4}) \quad (4)$$

The above equation gives the relation of the focal velocity versus the initial chirp  $\frac{dp}{d\xi}$  defined at a distance  $L$  before the focusing optics. In the high energy limit where  $1/\gamma^2 \ll (p_R/f_R) \left| \frac{dp}{d\xi} \right|^{-1}$ , the intra-beam velocity mismatch between slices can be neglected so that the  $O(\gamma^{-2})$  term can be dropped. In this situation, a constant  $\beta_f$  corresponds to a linear initial chirp. For a relatively small  $\gamma$ , e.g., proton or heavy ion beams, the spacing between beam slices will

change during the beam propagation due to the intra-beam velocity mismatch, therefore the chirp is  $L$ -dependent for a given  $\beta_f$ . If we define  $\frac{dp}{d\xi}$  at  $z = z_0$  ( $L = 0$ ), the focal velocity can be written as,

$$\beta_f \simeq 1 - \frac{p_R}{f_R} \left( \frac{dp}{d\xi} \right)^{-1} + \frac{1}{2\gamma^2} \left[ 1 - \frac{3p_R}{f_R} \left( \frac{dp}{d\xi} \right)^{-1} \right] + O(\gamma^{-4}). \quad (5)$$

### CHARACTERISTIC LENGTH OF THE FLYING FOCUS

The density distribution of the FF resembles a butterfly as shown in Fig. 1(b). It is important to quantitatively know the characteristic length within which the particles are well-focused. Considering a  $2f_R$  system, i.e., setting  $L = f_R$ , the transfer matrix of an arbitrary beam slice from the initial plane (denoted by “1”) to the focal plane (denoted by “2”) is [1]

$$M_{1 \rightarrow 2} = \begin{pmatrix} 1 - \frac{f_R}{f} & \frac{(2f - f_R)f_R}{f} \\ -1/f & 1 - \frac{f_R}{f} \end{pmatrix}, \quad (6)$$

where  $f_R$  is the focal length for the reference particle and  $f = f_R(1 + \delta)$  ( $\delta \equiv \frac{p - p_R}{p_R}$ ) for an arbitrary particle. Here we assume the inter-slice velocity mismatch is negligible and only consider the transverse motion. With the above transfer matrix, the evolution of the Twiss parameters from the initial plane to the focal plane is given by

$$\begin{pmatrix} \beta_T(\xi) \\ \alpha_T(\xi) \\ \gamma_T(\xi) \end{pmatrix}_2 = \begin{pmatrix} \frac{\delta^2}{(1 + \delta)^2} & -\frac{2\delta(1 + 2\delta)}{(1 + \delta)^2} f_R & \frac{(1 + 2\delta)^2}{(1 + \delta)^2} f_R^2 \\ -\frac{\delta}{f_R(1 + \delta)^2} & \frac{\delta^2 - 2\delta - 1}{(1 + \delta)^2} & -\frac{\delta(1 + 2\delta)}{(1 + \delta)^2} f_R \\ \frac{1}{f_R^2(1 + \delta)^2} & \frac{2\delta}{f_R(1 + \delta)^2} & \frac{\delta^2}{(1 + \delta)^2} \end{pmatrix} \begin{pmatrix} \beta_T \\ \alpha_T \\ \gamma_T \end{pmatrix}_1 \quad (7)$$

Here we have assumed that the Twiss parameters at the initial plane  $(\beta_T, \alpha_T, \gamma_T)_1$  are identical for each beam slice. For the reference particle  $\delta = 0$  and we can obtain from Eq. (7) that

$$\beta_{T,2}(\xi_R) = f_R^2 \gamma_{T,1}, \quad \alpha_{T,2}(\xi_R) = -\alpha_{T,1}, \quad \gamma_{T,2}(\xi_R) = \beta_{T,1}/f_R^2. \quad (8)$$

We assume  $\alpha_{T,2}(\xi_R) = 0$  at the focal plane and thus  $\alpha_{T,1}$  also vanishes. Substituting Eq. (8) into Eq. (7) and applying the relations  $\beta_T \epsilon = \sigma^2$  and  $\gamma_T \epsilon = \sigma'^2$  where  $\epsilon$  is the geometric emittance,  $\sigma$  is the beam size and  $\sigma'$  is the beam divergence, leads to an expression for the transverse size of each beam slice

$$\sigma^2(\xi) = \frac{\delta^2}{(1 + \delta)^2} f_R^2 \sigma_R'^2 + \frac{(1 + 2\delta)^2}{(1 + \delta)^2} \sigma_R^2. \quad (9)$$

Here  $\sigma_R \equiv \sigma(\xi_R)$  and  $\sigma_R' \equiv \sigma'(\xi_R)$ , and the subscript “2” has been omitted to simplify the denotation.

We define the characteristic length of the flying focus as the spacing between  $\xi_R$  and the slice position  $\xi_c$  where the spot size is doubled, i.e.,  $\sigma(\xi_c) = \sqrt{2}\sigma_R$ . Inserting this relation into the rhs of Eq. (9), we can derive an expression for the energy deviation at  $\xi_L$ ,

$$\delta(\xi_L) = \sqrt{\frac{\sigma_R^2}{2\sigma_R^2 + f_R^2 \sigma_R'^2}} = \sqrt{\frac{\beta^{*2}}{2\beta^{*2} + f_R^2}}. \quad (10)$$

where  $\beta^* = \sigma_R/\sigma_R'$ . For a linearly chirped beam with  $\delta(\xi) = h(\xi - \xi_R)$  where  $h$  is a constant coefficient, the characteristic length of the flying focal spot is

$$z_c \equiv |\xi_c - \xi_R| = \frac{1}{|h|} \sqrt{\frac{\beta^{*2}}{2\beta^{*2} + f_R^2}}. \quad (11)$$

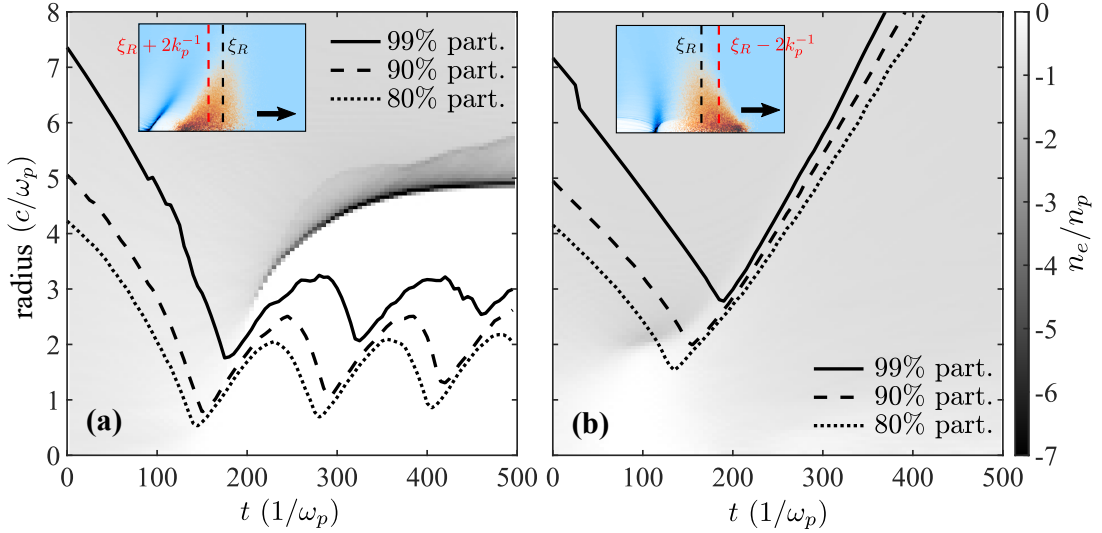

FIG. 2. Evolution of the tracked slice of drive beam and the plasma density distribution seen by this slice for (a) a negative-chirped beam and (b) a positive-chirped beam. The black and red dashed lines in the insets of both sub-figures represents the reference slice and the track one, respectively. The grey 2D plots reflects the evolution of the background electron density distribution seen by the tracked slice. The simulation parameters in (a) are identical to those Fig. 3(c), and those in (b) are identical to (a) except  $\beta_f = 0.995$ . The black arrows in the insets denote the beam propagation direction.

### GUIDING OF THE DRIVE BEAM WITH A SUPERLUMINAL VS. SUBLUMINAL FF

A subluminal FF does not lead to injection because the head of the beam does not remain guided. To illustrate the difference in guiding between a super- and sub-luminal FF, we tracked the evolution of a specific drive beam slice (red dashed lines in Fig. 2) at  $\xi = \xi_R + 2k_p^{-1}$  and of the plasma density seen by this slice. In a superluminal case shown in Fig. 2(a), as the FF moves forward from the beam tail, the size of the tracked slice initially decreases ( $\lesssim 200\omega_p^{-1}$ ) primarily due to the focusing from the wake. After the FF sweeps forward over the tracked slice, the wake excited by the fraction of beam in the front is now in the blowout regime and thus provides a strong focusing force to guide the entire beam behind it. Moreover, the blowout radius at the tracked slice quickly increases after the FF sweeps past it from  $200\omega_p^{-1} \lesssim t \lesssim 300\omega_p^{-1}$ . This process does not exist for a subluminal FF (a positive-chirped drive beam). This can be seen in Fig. 2(b), where we likewise tracked a beam slice at  $\xi = \xi_R - 2k_p^{-1}$  and the plasma density seen by it, as the FF now moves backwards. No clear ion channel forms for beam guiding and the observed slice quickly diffracts.

---

[1] S.-Y. Lee, *Accelerator physics* (World Scientific, 2004).
